# Supplementary material for: Herschel Galactic plane survey of [NII] fine structure emission
Source: arXiv:1510.05706 source file (2015-10-19)
Supplement: Supplementary file 1 [file appendixtable.pdf]

**Table 2.** Observed PACS integrated intensities for [N II] 122 $\mu$m and 205 $\mu$m transitions are tabulated together with the inferred electron volume densities and $N^+$ column densities. For each Line of Sight (LoS), we give the intensity in units of $10^{-8}$ $W m^{-2} sr$ averaged over the 25 PACS spaxels and accompanying uncertainty. The quantity $\sigma$ denotes the *rms* variation among the 25 spaxels at 122 $\mu$m wavelength.

| | | | [N II] 122$\mu$m | | | [N II] 205$\mu$m | | | |
|---|---|---|---|---|---|---|---|---|---|
| LoS Label | Longitude | OBSID | R$^{(a)}$ | Intensity ± (Err) | $\sigma$ | R$^{(a)}$ | Intensity ± (Err) | $n(e)$± (Err) | $N(N^+)$ ± (Err) |
| | | | | [$\times 10^{-8}$] [W m$^{-2}$sr$^{-1}$] | [$\times 10^{-8}$] | | [$\times 10^{-8}$] [W m$^{-2}$sr$^{-1}$] | cm$^{-3}$ | [$\times 10^{16}$] cm$^{-2}$ |
| G000.0+0.0 | 0.0000 | 1342265930 | (2) | 87.52 ± 0.383 | 18.13 | (2) | 25.05 ± 0.062 | 117.8 ± 1.0 | 33.6 ± 0.15 |
| G000.5+0.0 | 0.5000 | 1342265929 | (2) | 13.84 ± 0.082 | 3.97 | (2) | 7.09 ± 0.079 | 45.3 ± 0.9 | 10.7 ± 0.06 |
| G000.9+0.0 | 0.8696 | 1342265928 | (0) | ... ± ... | ... | (0) | ... ± ... | ... ± ... | ... ± ... |
| G001.7+0.0 | 1.7391 | 1342265927 | (3) | 0.97 ± 0.018 | 0.81 | (1) | <0.14 ± ... | ... ± ... | ... ± ... |
| G002.6+0.0 | 2.6087 | 1342265925 | (2) | 2.14 ± 0.015 | 0.50 | (2) | 1.45 ± 0.043 | 28.2 ± 1.5 | 2.6 ± 0.02 |
| G003.5+0.0 | 3.4783 | 1342265924 | (2) | 2.06 ± 0.025 | 0.42 | (3) | 1.77 ± 0.093 | 18.3 ± 1.9 | 4.0 ± 0.05 |
| G004.3+0.0 | 4.3478 | 1342265677 | (2) | 1.58 ± 0.017 | 0.57 | (3) | 1.15 ± 0.103 | 25.0 ± 4.0 | 2.2 ± 0.02 |
| G005.2+0.0 | 5.2174 | 1342265676 | (2) | 2.04 ± 0.017 | 0.62 | (2) | 2.35 ± 0.061 | 9.4 ± 0.7 | 8.2 ± 0.07 |
| G006.1+0.0 | 6.0870 | 1342265675 | (2) | 3.93 ± 0.028 | 0.54 | (3) | 2.75 ± 0.069 | 26.8 ± 1.2 | 5.0 ± 0.04 |
| G007.0+0.0 | 6.9565 | 1342265674 | (2) | 7.78 ± 0.035 | 1.38 | (2) | 4.54 ± 0.045 | 36.6 ± 0.7 | 7.3 ± 0.03 |
| G007.8+0.0 | 7.8261 | 1342265673 | (2) | 2.49 ± 0.018 | 0.59 | (3) | 1.78 ± 0.087 | 25.7 ± 2.3 | 3.3 ± 0.02 |
| G008.7+0.0 | 8.6957 | 1342265672 | (2) | 3.73 ± 0.016 | 0.41 | (2) | 3.56 ± 0.060 | 14.7 ± 0.5 | 9.1 ± 0.04 |
| G009.6+0.0 | 9.5652 | 1342265698 | (2) | 0.93 ± 0.017 | 0.39 | (3) | 0.66 ± 0.066 | 25.8 ± 4.7 | 1.2 ± 0.02 |
| G010.4+0.0 | 10.4348 | 1342265671 | (2) | 8.11 ± 0.051 | 3.15 | (2) | 5.05 ± 0.057 | 32.8 ± 0.7 | 8.5 ± 0.05 |
| G011.3+0.0 | 11.3043 | 1342265923 | (2) | 2.78 ± 0.020 | 0.43 | (2) | 3.16 ± 0.061 | 9.8 ± 0.5 | 10.7 ± 0.08 |
| G012.2+0.0 | 12.1739 | 1342265670 | (2) | 8.15 ± 0.038 | 1.12 | (2) | 5.45 ± 0.070 | 29.0 ± 0.7 | 9.7 ± 0.05 |
| G013.0+0.0 | 13.0435 | 1342265921 | (2) | 3.56 ± 0.023 | 0.96 | (2) | 2.08 ± 0.091 | 36.6 ± 2.7 | 3.4 ± 0.02 |
| G013.9+0.0 | 13.9130 | 1342265922 | (2) | 5.01 ± 0.023 | 0.43 | (2) | 3.49 ± 0.099 | 27.0 ± 1.4 | 6.4 ± 0.03 |
| G014.8+0.0 | 14.7826 | 1342267877 | (2) | 4.06 ± 0.026 | 0.45 | (2) | 3.15 ± 0.058 | 22.2 ± 0.8 | 6.3 ± 0.04 |
| G015.7+0.0 | 15.6522 | 1342267878 | (2) | 1.05 ± 0.010 | 0.38 | (3) | 0.90 ± 0.051 | 18.6 ± 2.1 | 2.0 ± 0.02 |
| G016.5+0.0 | 16.5217 | 1342267881 | (2) | 3.79 ± 0.025 | 0.57 | (3) | 2.19 ± 0.041 | 37.1 ± 1.2 | 3.5 ± 0.02 |
| G017.4+0.0 | 17.3913 | 1342267879 | (3) | 1.15 ± 0.012 | 1.02 | (3) | 0.78 ± 0.064 | 28.1 ± 4.1 | 1.4 ± 0.01 |
| G018.3+0.0 | 18.2609 | 1342267880 | (2) | 2.92 ± 0.027 | 0.60 | (3) | 2.45 ± 0.050 | 19.2 ± 0.8 | 5.3 ± 0.05 |
| G019.1+0.0 | 19.1304 | 1342267844 | (2) | 0.71 ± 0.013 | 0.31 | (2) | 0.75 ± 0.042 | 11.7 ± 1.6 | 2.2 ± 0.04 |
| G020.0+0.0 | 20.0000 | 1342267843 | (2) | 1.72 ± 0.019 | 0.43 | (3) | 1.72 ± 0.055 | 13.3 ± 1.0 | 4.7 ± 0.05 |
| G020.9+0.0 | 20.8696 | 1342267842 | (2) | 5.20 ± 0.028 | 0.99 | (2) | 3.36 ± 0.067 | 30.8 ± 1.1 | 5.8 ± 0.03 |
| G021.7+0.0 | 21.7391 | 1342266922 | (2) | 6.57 ± 0.038 | 0.65 | (2) | 4.50 ± 0.058 | 27.9 ± 0.7 | 8.1 ± 0.05 |
| G023.5+0.0 | 23.4783 | 1342254216 | (2) | 14.76 ± 0.053 | 1.52 | (2) | 9.39 ± 0.056 | 31.7 ± 0.4 | 16.0 ± 0.06 |
| G024.3+0.0 | 24.3478 | 1342267626 | (2) | 8.47 ± 0.067 | 0.63 | (2) | 6.44 ± 0.048 | 23.1 ± 0.5 | 12.7 ± 0.10 |
| G025.2+0.0 | 25.2174 | 1342254217 | (2) | 4.97 ± 0.032 | 0.71 | (2) | 4.83 ± 0.055 | 14.2 ± 0.4 | 12.7 ± 0.08 |
| G026.1+0.0 | 26.0870 | 1342254218 | (2) | 18.41 ± 0.083 | 3.90 | (2) | 9.03 ± 0.077 | 48.6 ± 0.8 | 13.4 ± 0.06 |
| G027.0+0.0 | 26.9565 | 1342254255 | (2) | 3.90 ± 0.028 | 0.44 | (2) | 2.98 ± 0.090 | 22.8 ± 1.3 | 5.9 ± 0.04 |
| G027.8+0.0 | 27.8261 | 1342254219 | (2) | 1.92 ± 0.023 | 0.40 | (2) | 1.62 ± 0.094 | 18.9 ± 2.2 | 3.6 ± 0.04 |
| G028.7+0.0 | 28.6957 | 1342254256 | (2) | 11.12 ± 0.035 | 0.73 | (2) | 6.11 ± 0.070 | 40.4 ± 0.8 | 9.6 ± 0.03 |
| G030.0+0.0 | 30.0000 | 1342254257 | (2) | 6.56 ± 0.028 | 0.77 | (2) | 4.35 ± 0.088 | 29.4 ± 1.0 | 7.7 ± 0.03 |
| G031.3+0.0 | 31.2766 | 1342254274 | (2) | 10.37 ± 0.045 | 0.89 | (2) | 6.65 ± 0.060 | 31.2 ± 0.5 | 11.4 ± 0.05 |
| G032.6+0.0 | 32.5532 | 1342254275 | (2) | 1.88 ± 0.015 | 0.31 | (3) | 1.07 ± 0.074 | 38.0 ± 4.4 | 1.7 ± 0.01 |
| G033.8+0.0 | 33.8298 | 1342254297 | (2) | 1.49 ± 0.012 | 0.43 | (2) | 1.31 ± 0.072 | 17.5 ± 2.0 | 3.0 ± 0.02 |
| G035.1+0.0 | 35.1064 | 1342254298 | (2) | 1.60 ± 0.013 | 0.40 | (2) | 1.15 ± 0.051 | 25.4 ± 2.0 | 2.2 ± 0.02 |
| G036.4+0.0 | 36.3830 | 1342254606 | (2) | 1.85 ± 0.012 | 0.39 | (2) | 1.51 ± 0.091 | 20.2 ± 2.3 | 3.2 ± 0.02 |
| G037.7+0.0 | 37.6596 | 1342254299 | (2) | 5.00 ± 0.025 | 0.80 | (2) | 4.19 ± 0.062 | 19.2 ± 0.6 | 9.1 ± 0.05 |
| G038.9+0.0 | 38.9362 | 1342254607 | (3) | 0.45 ± 0.017 | 0.30 | (1) | <0.21 ± ... | ... ± ... | ... ± ... |
| G040.2+0.0 | 40.2128 | 1342254300 | (2) | 0.44 ± 0.015 | 0.31 | (3) | 0.65 ± 0.068 | 3.8 ± 2.0 | 4.9 ± 0.16 |
| G041.5+0.0 | 41.4894 | 1342254608 | (2) | 2.41 ± 0.018 | 0.72 | (3) | 1.39 ± 0.050 | 37.5 ± 2.3 | 2.2 ± 0.02 |
| G042.8+0.0 | 42.7660 | 1342254609 | (2) | 0.91 ± 0.010 | 0.39 | (1) | <0.21 ± ... | ... ± ... | ... ± ... |
| G044.0+0.0 | 44.0426 | 1342254610 | (2) | 1.49 ± 0.014 | 0.51 | (3) | 1.50 ± 0.097 | 13.1 ± 1.9 | 4.1 ± 0.04 |
| G045.3+0.0 | 45.3191 | 1342254611 | (2) | 0.82 ± 0.011 | 0.33 | (3) | 0.52 ± 0.060 | 31.5 ± 6.2 | 0.9 ± 0.01 |
| G046.6+0.0 | 46.5957 | 1342254612 | (2) | 0.95 ± 0.015 | 0.39 | (1) | <0.24 ± ... | ... ± ... | ... ± ... |
| G047.9+0.0 | 47.8723 | 1342254616 | (3) | 0.42 ± 0.008 | 0.29 | (1) | <0.13 ± ... | ... ± ... | ... ± ... |
| G049.1+0.0 | 49.1489 | 1342254617 | (2) | 1.70 ± 0.010 | 0.49 | (2) | 1.38 ± 0.079 | 20.3 ± 2.2 | 2.9 ± 0.02 |
| G050.4+0.0 | 50.4255 | 1342254618 | (3) | 0.39 ± 0.014 | 0.24 | (1) | <0.24 ± ... | ... ± ... | ... ± ... |
| G051.7+0.0 | 51.7021 | 1342254619 | (3) | 0.21 ± 0.008 | 0.09 | (1) | <0.15 ± ... | ... ± ... | ... ± ... |
| G053.0+0.0 | 52.9787 | 1342254620 | (3) | 0.27 ± 0.011 | 0.15 | (1) | <0.16 ± ... | ... ± ... | ... ± ... |
| G054.3+0.0 | 54.2553 | 1342254767 | (2) | 1.32 ± 0.012 | 0.40 | (2) | 0.51 ± 0.047 | 69.9 ± 10.5 | 0.7 ± 0.01 |
| G055.5+0.0 | 55.5319 | 1342254768 | (3) | 0.14 ± 0.012 | 0.02 | (1) | <0.18 ± ... | ... ± ... | ... ± ... |
| G056.8+0.0 | 56.8085 | 1342254769 | (1) | <0.04 ± ... | ... | (1) | <0.19 ± ... | ... ± ... | ... ± ... |
| G058.1+0.0 | 58.0851 | 1342254770 | (1) | <0.04 ± ... | ... | (1) | <0.12 ± ... | ... ± ... | ... ± ... |
| G060.0+0.0 | 60.0000 | 1342256254 | (3) | 0.41 ± 0.011 | 0.28 | (1) | <0.23 ± ... | ... ± ... | ... ± ... |
| G064.5+0.0 | 64.5283 | 1342256255 | (1) | <0.04 ± ... | ... | (1) | <0.18 ± ... | ... ± ... | ... ± ... |
| G069.1+0.0 | 69.0566 | 1342256256 | (1) | <0.06 ± ... | ... | (1) | <0.24 ± ... | ... ± ... | ... ± ... |
| G073.6+0.0 | 73.5849 | 1342257793 | (1) | <0.08 ± ... | ... | (1) | <0.23 ± ... | ... ± ... | ... ± ... |
| G078.1+0.0 | 78.1132 | 1342256763 | (2) | 1.13 ± 0.013 | 0.37 | (2) | 1.14 ± 0.063 | 13.0 ± 1.7 | 3.2 ± 0.04 |
| G082.6+0.0 | 82.6415 | 1342259608 | (1) | <0.02 ± ... | ... | (1) | <0.20 ± ... | ... ± ... | ... ± ... |
| G087.2+0.0 | 87.1698 | 1342262028 | (3) | 0.14 ± 0.007 | 0.02 | (1) | <0.15 ± ... | ... ± ... | ... ± ... |
| G091.7+0.0 | 91.6981 | 1342256766 | (1) | <0.04 ± ... | ... | (1) | <0.21 ± ... | ... ± ... | ... ± ... |
| G096.2+0.0 | 96.2264 | 1342257686 | (1) | <0.04 ± ... | ... | (1) | <0.12 ± ... | ... ± ... | ... ± ... |
| G109.8+0.0 | 109.8113 | 1342262544 | (1) | <0.03 ± ... | ... | (1) | <0.15 ± ... | ... ± ... | ... ± ... |
| G114.3+0.0 | 114.3396 | 1342263496 | (1) | <0.03 ± ... | ... | (1) | <0.22 ± ... | ... ± ... | ... ± ... |
| G127.9+0.0 | 127.9245 | 1342265699 | (1) | <0.03 ± ... | ... | (1) | <0.16 ± ... | ... ± ... | ... ± ... |
| G132.5+0.0 | 132.4528 | 1342265445 | (1) | <0.03 ± ... | ... | (1) | <0.18 ± ... | ... ± ... | ... ± ... |

[a] Detection status, with the meanings (1): non-detection, (2): detection in individual spaxel or spaxels, and (3): only the average of all spaxels provides a detection. For the non-detections, we give the $3\sigma$ upper limits on the intensities.

**Table 3.** PACS results (continued)

| | | | [N II] 122$\mu$m | | | [N II] 205$\mu$m | | | |
|---|---|---|---|---|---|---|---|---|---|
| LoS Label | Longitude | OBSID | R[(a)] | Intensity ± (Err) | $\sigma$ | R[(a)] | Intensity ± (Err) | $n(e)$± (Err) | $N(N^+)$ ± (Err) |
| | | | | [$\times 10^{-8}$] [W m$^{-2}$sr$^{-1}$] | [$\times 10^{-8}$] | | [$\times 10^{-8}$] [W m$^{-2}$sr$^{-1}$] | cm$^{-3}$ | [$\times 10^{16}$] cm$^{-2}$ |
| G146.0+0.0 | 146.0377 | 1342265446 | (1) | <0.04 ± ... | ... | (1) | <0.13 ± ... | ... ± ... | ... ± ... |
| G150.6+0.0 | 150.5660 | 1342265700 | (1) | <0.03 ± ... | ... | (1) | <0.17 ± ... | ... ± ... | ... ± ... |
| G164.2+0.0 | 164.1509 | 1342265952 | (1) | <0.03 ± ... | ... | (3) | 0.55 ± 0.053 | ... ± ... | ... ± ... |
| G168.7+0.0 | 168.6792 | 1342267858 | (1) | <0.03 ± ... | ... | (3) | 0.42 ± 0.041 | ... ± ... | ... ± ... |
| G184.5+0.0 | 184.5283 | 1342267859 | (1) | <0.03 ± ... | ... | (1) | <0.12 ± ... | ... ± ... | ... ± ... |
| G189.1+0.0 | 189.0570 | 1342267860 | (1) | <0.03 ± ... | ... | (1) | <0.12 ± ... | ... ± ... | ... ± ... |
| G202.6+0.0 | 202.6420 | 1342250904 | (1) | <0.03 ± ... | ... | (1) | <0.16 ± ... | ... ± ... | ... ± ... |
| G207.2+0.0 | 207.1700 | 1342267861 | (1) | <0.05 ± ... | ... | (2) | 0.47 ± 0.048 | ... ± ... | ... ± ... |
| G220.8+0.0 | 220.7550 | 1342251176 | (1) | <0.03 ± ... | ... | (1) | <0.14 ± ... | ... ± ... | ... ± ... |
| G225.3+0.0 | 225.2830 | 1342251177 | (1) | <0.03 ± ... | ... | (1) | <0.10 ± ... | ... ± ... | ... ± ... |
| G238.9+0.0 | 238.8680 | 1342254932 | (1) | <0.04 ± ... | ... | (1) | <0.16 ± ... | ... ± ... | ... ± ... |
| G243.4+0.0 | 243.3960 | 1342254931 | (1) | <0.03 ± ... | ... | (1) | <0.16 ± ... | ... ± ... | ... ± ... |
| G252.5+0.0 | 252.4530 | 1342256248 | (1) | <0.03 ± ... | ... | (1) | <0.15 ± ... | ... ± ... | ... ± ... |
| G257.0+0.0 | 256.9810 | 1342256783 | (1) | <0.02 ± ... | ... | (1) | <0.15 ± ... | ... ± ... | ... ± ... |
| G261.5+0.0 | 261.5090 | 1342256784 | (1) | <0.03 ± ... | ... | (1) | <0.22 ± ... | ... ± ... | ... ± ... |
| G266.0+0.0 | 266.0380 | 1342257275 | (1) | <0.04 ± ... | ... | (1) | <0.20 ± ... | ... ± ... | ... ± ... |
| G270.6+0.0 | 270.5660 | 1342249384 | (1) | <0.03 ± ... | ... | (1) | <0.12 ± ... | ... ± ... | ... ± ... |
| G275.1+0.0 | 275.0940 | 1342249385 | (1) | <0.03 ± ... | ... | (1) | <0.12 ± ... | ... ± ... | ... ± ... |
| G279.6+0.0 | 279.6230 | 1342249386 | (1) | <0.04 ± ... | ... | (1) | <0.13 ± ... | ... ± ... | ... ± ... |
| G284.2+0.0 | 284.1510 | 1342249387 | (3) | 0.62 ± 0.013 | 0.48 | (1) | <0.17 ± ... | ... ± ... | ... ± ... |
| G288.7+0.0 | 288.6790 | 1342249390 | (3) | 0.14 ± 0.010 | 0.02 | (1) | <0.16 ± ... | ... ± ... | ... ± ... |
| G293.2+0.0 | 293.2080 | 1342249391 | (1) | <0.03 ± ... | ... | (1) | <0.13 ± ... | ... ± ... | ... ± ... |
| G300.0+0.0 | 300.0000 | 1342249392 | (3) | 0.21 ± 0.012 | 0.07 | (1) | <0.18 ± ... | ... ± ... | ... ± ... |
| G301.3+0.0 | 301.2770 | 1342249393 | (3) | 0.36 ± 0.011 | 0.22 | (1) | <0.22 ± ... | ... ± ... | ... ± ... |
| G302.6+0.0 | 302.5530 | 1342263462 | (2) | 2.35 ± 0.015 | 0.40 | (3) | 2.22 ± 0.076 | 15.0 ± 1.1 | 5.6 ± 0.04 |
| G303.8+0.0 | 303.8300 | 1342263463 | (2) | 1.10 ± 0.012 | 0.33 | (3) | 0.67 ± 0.072 | 33.8 ± 6.1 | 1.1 ± 0.01 |
| G305.1+0.0 | 305.1060 | 1342266978 | (2) | 13.80 ± 0.050 | 4.20 | (2) | 6.19 ± 0.064 | 56.1 ± 1.0 | 8.9 ± 0.03 |
| G306.4+0.0 | 306.3830 | 1342266976 | (2) | 0.94 ± 0.012 | 0.47 | (3) | 1.13 ± 0.088 | 8.4 ± 1.9 | 4.3 ± 0.05 |
| G307.7+0.0 | 307.6600 | 1342266974 | (2) | 2.48 ± 0.011 | 0.34 | (2) | 2.18 ± 0.061 | 17.5 ± 1.0 | 5.0 ± 0.02 |
| G308.9+0.0 | 308.9360 | 1342266972 | (2) | 1.29 ± 0.013 | 0.27 | (3) | 0.50 ± 0.058 | 70.3 ± 13.2 | 0.7 ± 0.01 |
| G310.2+0.0 | 310.2130 | 1342266970 | (2) | 1.00 ± 0.013 | 0.40 | (3) | 0.51 ± 0.053 | 45.5 ± 7.8 | 0.8 ± 0.01 |
| G311.5+0.0 | 311.4890 | 1342266968 | (2) | 1.60 ± 0.017 | 0.35 | (3) | 1.27 ± 0.052 | 21.3 ± 1.7 | 2.6 ± 0.03 |
| G312.8+0.0 | 312.7660 | 1342266964 | (2) | 1.72 ± 0.016 | 0.36 | (3) | 1.27 ± 0.072 | 24.2 ± 2.5 | 2.5 ± 0.02 |
| G314.0+0.0 | 314.0430 | 1342267177 | (2) | 1.88 ± 0.020 | 0.53 | (3) | 1.34 ± 0.050 | 26.2 ± 1.8 | 2.5 ± 0.03 |
| G315.3+0.0 | 315.3190 | 1342267179 | (3) | 0.37 ± 0.012 | 0.22 | (1) | <0.25 ± ... | ... ± ... | ... ± ... |
| G316.6+0.0 | 316.5960 | 1342267182 | (2) | 5.63 ± 0.032 | 0.56 | (2) | 4.33 ± 0.062 | 22.7 ± 0.6 | 8.6 ± 0.05 |
| G317.9+0.0 | 317.8720 | 1342267184 | (2) | 4.06 ± 0.023 | 0.56 | (2) | 2.80 ± 0.070 | 27.6 ± 1.2 | 5.1 ± 0.03 |
| G319.1+0.0 | 319.1490 | 1342267186 | (2) | 0.78 ± 0.019 | 0.28 | (3) | 0.52 ± 0.060 | 29.0 ± 5.9 | 0.9 ± 0.02 |
| G320.4+0.0 | 320.4250 | 1342266982 | (1) | <0.23 ± ... | ... | (2) | 1.02 ± 0.054 | ... ± ... | ... ± ... |
| G321.7+0.0 | 321.7020 | 1342266981 | (3) | 0.66 ± 0.014 | 0.52 | (3) | 0.55 ± 0.052 | 19.6 ± 3.6 | 1.2 ± 0.02 |
| G323.0+0.0 | 322.9790 | 1342266979 | (3) | 0.31 ± 0.011 | 0.18 | (1) | <0.33 ± ... | ... ± ... | ... ± ... |
| G324.3+0.0 | 324.2550 | 1342266977 | (3) | 0.67 ± 0.013 | 0.54 | (1) | <0.15 ± ... | ... ± ... | ... ± ... |
| G326.8+0.0 | 326.8080 | 1342266975 | (2) | 10.03 ± 0.032 | 1.03 | (2) | 6.12 ± 0.068 | 33.9 ± 0.7 | 10.2 ± 0.03 |
| G328.1+0.0 | 328.0850 | 1342266973 | (2) | 2.10 ± 0.023 | 0.40 | (3) | 1.41 ± 0.061 | 28.8 ± 2.2 | 2.5 ± 0.03 |
| G330.0+0.0 | 330.0000 | 1342266971 | (2) | 1.47 ± 0.018 | 0.43 | (2) | 0.96 ± 0.056 | 30.3 ± 3.1 | 1.7 ± 0.02 |
| G330.9+0.0 | 330.8700 | 1342266969 | (2) | 1.60 ± 0.022 | 0.60 | (1) | <0.19 ± ... | ... ± ... | ... ± ... |
| G331.7+0.0 | 331.7390 | 1342267183 | (2) | 4.94 ± 0.041 | 0.63 | (2) | 3.54 ± 0.085 | 25.7 ± 1.2 | 6.6 ± 0.05 |
| G332.6+0.0 | 332.6090 | 1342265940 | (2) | 4.59 ± 0.026 | 0.63 | (2) | 2.79 ± 0.082 | 34.2 ± 1.7 | 4.6 ± 0.03 |
| G333.5+0.0 | 333.4780 | 1342265939 | (2) | 9.25 ± 0.018 | 0.93 | (2) | 5.05 ± 0.054 | 40.8 ± 0.7 | 7.9 ± 0.02 |
| G334.3+0.0 | 334.3480 | 1342265938 | (2) | 1.61 ± 0.012 | 0.50 | (3) | 1.36 ± 0.065 | 18.7 ± 1.8 | 3.0 ± 0.02 |
| G335.2+0.0 | 335.2170 | 1342265937 | (2) | 3.32 ± 0.018 | 0.34 | (2) | 2.90 ± 0.060 | 17.6 ± 0.8 | 6.7 ± 0.04 |
| G336.1+0.0 | 336.0870 | 1342265936 | (2) | 14.92 ± 0.074 | 2.21 | (2) | 9.63 ± 0.065 | 30.8 ± 0.4 | 16.6 ± 0.08 |
| G337.0+0.0 | 336.9570 | 1342265697 | (2) | 16.76 ± 0.083 | 1.88 | (2) | 11.06 ± 0.082 | 29.7 ± 0.5 | 19.4 ± 0.10 |
| G337.8+0.0 | 337.8260 | 1342265692 | (2) | 12.25 ± 0.041 | 2.05 | (2) | 8.16 ± 0.071 | 29.2 ± 0.5 | 14.4 ± 0.05 |
| G338.7+0.0 | 338.6960 | 1342265691 | (2) | 3.37 ± 0.023 | 0.39 | (3) | 2.20 ± 0.070 | 30.2 ± 1.7 | 3.8 ± 0.03 |
| G339.6+0.0 | 339.5650 | 1342265690 | (2) | 2.36 ± 0.013 | 0.54 | (3) | 2.16 ± 0.100 | 16.1 ± 1.6 | 5.2 ± 0.03 |
| G340.4+0.0 | 340.4350 | 1342265689 | (2) | 4.10 ± 0.034 | 0.75 | (2) | 3.34 ± 0.114 | 20.3 ± 1.4 | 7.1 ± 0.06 |
| G341.3+0.0 | 341.3040 | 1342265688 | (2) | 1.83 ± 0.020 | 0.41 | (3) | 1.23 ± 0.079 | 29.0 ± 3.3 | 2.2 ± 0.02 |
| G342.2+0.0 | 342.1740 | 1342265687 | (2) | 4.65 ± 0.030 | 0.64 | (2) | 4.58 ± 0.042 | 13.8 ± 0.3 | 12.2 ± 0.08 |
| G343.0+0.0 | 343.0430 | 1342265686 | (2) | 3.13 ± 0.018 | 0.43 | (2) | 2.47 ± 0.075 | 21.5 ± 1.2 | 5.1 ± 0.03 |
| G343.9+0.0 | 343.9130 | 1342265685 | (2) | 3.73 ± 0.025 | 0.37 | (2) | 2.46 ± 0.052 | 29.7 ± 1.1 | 4.3 ± 0.03 |
| G344.8+0.0 | 344.7830 | 1342267185 | (2) | 1.37 ± 0.020 | 0.42 | (3) | 0.80 ± 0.056 | 36.4 ± 4.3 | 1.3 ± 0.02 |
| G345.7+0.0 | 345.6520 | 1342267869 | (2) | 12.60 ± 0.044 | 7.55 | (2) | 5.44 ± 0.081 | 59.6 ± 1.5 | 7.7 ± 0.03 |
| G346.5+0.0 | 346.5220 | 1342267178 | (2) | 2.90 ± 0.020 | 0.77 | (2) | 1.71 ± 0.059 | 36.0 ± 2.1 | 2.8 ± 0.02 |
| G347.4+0.0 | 347.3910 | 1342264238 | (2) | 1.92 ± 0.013 | 0.54 | (3) | 1.32 ± 0.049 | 27.5 ± 1.8 | 2.4 ± 0.02 |
| G348.3+0.0 | 348.2610 | 1342264237 | (2) | 3.02 ± 0.020 | 0.90 | (2) | 2.07 ± 0.064 | 27.7 ± 1.5 | 3.7 ± 0.02 |
| G349.1+0.0 | 349.1300 | 1342267870 | (2) | 21.31 ± 0.096 | 4.41 | (2) | 8.67 ± 0.057 | 65.7 ± 0.8 | 12.1 ± 0.05 |
| G350.0+0.0 | 350.0000 | 1342265935 | (3) | 0.36 ± 0.008 | 0.23 | (1) | <0.22 ± ... | ... ± ... | ... ± ... |
| G350.9+0.0 | 350.8700 | 1342265684 | (2) | 1.42 ± 0.013 | 0.41 | (2) | 1.22 ± 0.069 | 18.1 ± 2.1 | 2.8 ± 0.03 |
| G351.7+0.0 | 351.7390 | 1342265683 | (2) | 1.61 ± 0.025 | 0.48 | (3) | 1.68 ± 0.055 | 12.1 ± 1.0 | 4.9 ± 0.07 |
| G352.6+0.0 | 352.6090 | 1342265682 | (2) | 1.47 ± 0.021 | 0.36 | (3) | 1.22 ± 0.055 | 19.6 ± 1.8 | 2.6 ± 0.04 |
| G353.5+0.0 | 353.4780 | 1342265681 | (2) | 3.68 ± 0.027 | 0.62 | (2) | 2.95 ± 0.066 | 20.9 ± 0.9 | 6.1 ± 0.04 |
| G354.3+0.0 | 354.3480 | 1342265680 | (2) | 2.33 ± 0.020 | 0.65 | (2) | 1.53 ± 0.048 | 29.9 ± 1.7 | 2.7 ± 0.02 |
| G355.2+0.0 | 355.2170 | 1342267874 | (2) | 5.22 ± 0.017 | 1.34 | (2) | 1.87 ± 0.060 | 80.5 ± 4.2 | 2.6 ± 0.01 |
| G356.1+0.0 | 356.0870 | 1342265934 | (2) | 2.59 ± 0.020 | 0.31 | (3) | 1.63 ± 0.038 | 32.3 ± 1.4 | 2.8 ± 0.02 |
| G357.0+0.0 | 356.9570 | 1342265933 | (3) | 0.35 ± 0.010 | 0.21 | (1) | <0.18 ± ... | ... ± ... | ... ± ... |
| G357.8+0.0 | 357.8260 | 1342265932 | (2) | 0.82 ± 0.020 | 0.31 | (1) | <0.19 ± ... | ... ± ... | ... ± ... |
| G358.7+0.0 | 358.6960 | 1342267875 | (0) | ... ± ... | ... | (0) | ... ± ... | ... ± ... | ... ± ... |
| G359.5+0.0 | 359.5000 | 1342265931 | (2) | 17.30 ± 0.102 | 1.69 | (2) | 9.16 ± 0.095 | 42.9 ± 0.8 | 14.1 ± 0.08 |
